# Supplementary material for: DiQAD: A Benchmark Dataset for End-to-End Open-domain Dialogue Assessment
Source: arXiv:2310.16319 source file (2023-10-25)
Supplement: Supplementary file 1 [file 6-appendix.tex]

\appendix

\section{Example Appendix}
\label{sec:appendix}

This is an appendix.

\begin{table}[!t]\centering\small
\setlength\tabcolsep{2pt}
\begin{tabular}{@{}l cccccccc@{}}
\toprule
& Params & Layer & Heads & Hidden & Train & Test & Acc\\
\midrule
Xbase & 296M & 20	& 16	& 1024	&  \\
Base & 118M & 12	& 12 & 768	& \\
Medium & 75M & 6	& 12	& 768	&  \\
Mini & 27M	& 6	& 12	& 384	&  \\
Micro & 23M & 4 & 12 & 384\\
Nano & 18M  & 4 & 12 & 312\\
\bottomrule
\end{tabular}
\caption{Model size.}\label{table:model-selection}
\end{table}
